# Supplementary material for: The influence of supernova remnants on the interstellar medium in the Large Magellanic Cloud seen at 20--600 $\mu$m wavelengths
Source: arXiv:1410.5709 source file (2015-03-06)
Supplement: Supplementary file 1 [file Appendix1.pdf]

Draft version October 20, 2014
Preprint typeset using LaTeX style emulateapj v. 05/12/14

# THE INFLUENCE OF SUPERNOVA REMNANTS ON THE INTERSTELLAR MEDIUM IN THE LARGE MAGELLANIC CLOUD SEEN AT 20–600 $\mu$M WAVELENGTHS

Maša Lakićević[1], Jacco Th. van Loon[1], Margaret Meixner[2,3], Karl Gordon[2,4], Caroline Bot[5], Julia Roman-Duval[2], Brian Babler[6], Alberto Bolatto[7], Chad Engelbracht[8], Miroslav Filipović[9], Sacha Hony[10], Remy Indebetouw[11,12], Karl Misselt[8], Edward Montiel[8,13], K. Okumura[10], Pasquale Panuzzo[10,14], Ferdinando Patat[15], Marc Sauvage[10], Jonathan Seale[2,16], George Sonneborn[17], Tea Temim[17,18], Dejan Urošević[19,20], & Giovanna Zanardo[21]

(Received August 2014; Revised September 2014; Accepted 2014?)

*Subject headings:*

## 1. HERE WE PROVIDE THE ADDITIONAL IMAGES TO BE AVAILABLE ONLY ONLINE

## APPENDIX

## A. ATLAS OF SNRS IN THE LARGE MAGELLANIC CLOUDS: MAPS OF DUST MASS AND TEMPERATURE

Here we give the maps of dust mass and temperature in and around of SNRs in the LMC made using *Herschel* images at 100−500 $\mu$m. We present all the remnants that were given in the paper *The influence of supernova remnants on the interstellar medium in the Large Magellanic Cloud seen at 20–600 $\mu$m wavelengths*, but their maps were not shown there. For each remnant on the left side is the mass map and on the right side the temperature map. The main conclusion based on these maps was that the SNRs remove and heat up the dust, since we notice that often there is less dust seen towards SNRs than in their surroundings and that the dust within SNRs is often warmer.

[1] Lennard-Jones Laboratories, Keele University, ST5 5BG, UK; m.lakicevic@keele.ac.uk
[2] Space Telescope Science Institute, 3700 San Martin Dr., Baltimore, MD 21218, USA
[3] Department of Physics and Astronomy, Johns Hopkins University, 366 Bloomberg Center, 3400 N. Charles Street, Baltimore, MD 21218, USA
[4] Sterrenkundig Observatorium, Universiteit Gent, Gent, Belgium
[5] Observatoire astronomique de Strasbourg, Université de Strasbourg, CNRS, UMR 7550, 11 rue de l'université, F-67000 Strasbourg, France
[6] Department of Astronomy, 475 North Charter St., University of Wisconsin, Madison, WI 53706, USA
[7] Laboratory of Millimeter Astronomy, University of Maryland, College Park, MD 29742, USA
[8] Steward Observatory, University of Arizona, 933 North Cherry Ave., Tucson, AZ 85721, USA
[9] University of Western Sydney, Locked Bag 1797, Penrith South DC, NSW 1797, Australia
[10] CEA, Laboratoire AIM, Irfu/SAp, Orme des Merisiers, F-91191 Gif-sur-Yvette, France
[11] Department of Astronomy, University of Virginia, P.O. Box 400325, Charlottesville, VA 22903, USA
[12] National Radio Astronomy Observatory, 520 Edgemont Road, Charlottesville, VA 22903, USA
[13] Louisiana State University, Department of Physics & Astronomy, 233-A Nicholson Hall, Tower Dr., Baton Rouge, LA 70803, USA
[14] CNRS, Observatoire de Paris - Lab. GEPI, Bat. 11, 5, place Jules Janssen, 92195 Meudon CEDEX, France
[15] European Organization for Astronomical Research in the Southern Hemisphere (ESO), Karl-Schwarzschild-Straße 2, 85748 Garching bei München, Germany
[16] The Johns Hopkins University, Department of Physics and Astronomy, 366 Bloomberg Center, 3400 N. Charles Street, Baltimore, MD 21218, USA
[17] NASA Goddard Space Flight Center, Code 665, Greenbelt, MD 20771, USA
[18] CRESST, University of Maryland, College Park, MD 20742, USA
[19] Department of Astronomy, Faculty of Mathematics, University of Belgrade, Studentski trg 16, 11000 Belgrade, Serbia
[20] Isaac Newton Institute of Chile, Yugoslavia Branch
[21] International Centre for Radio Astronomy Research (ICRAR), M468, University of Western Australia, Crawley, WA 6009, Australia

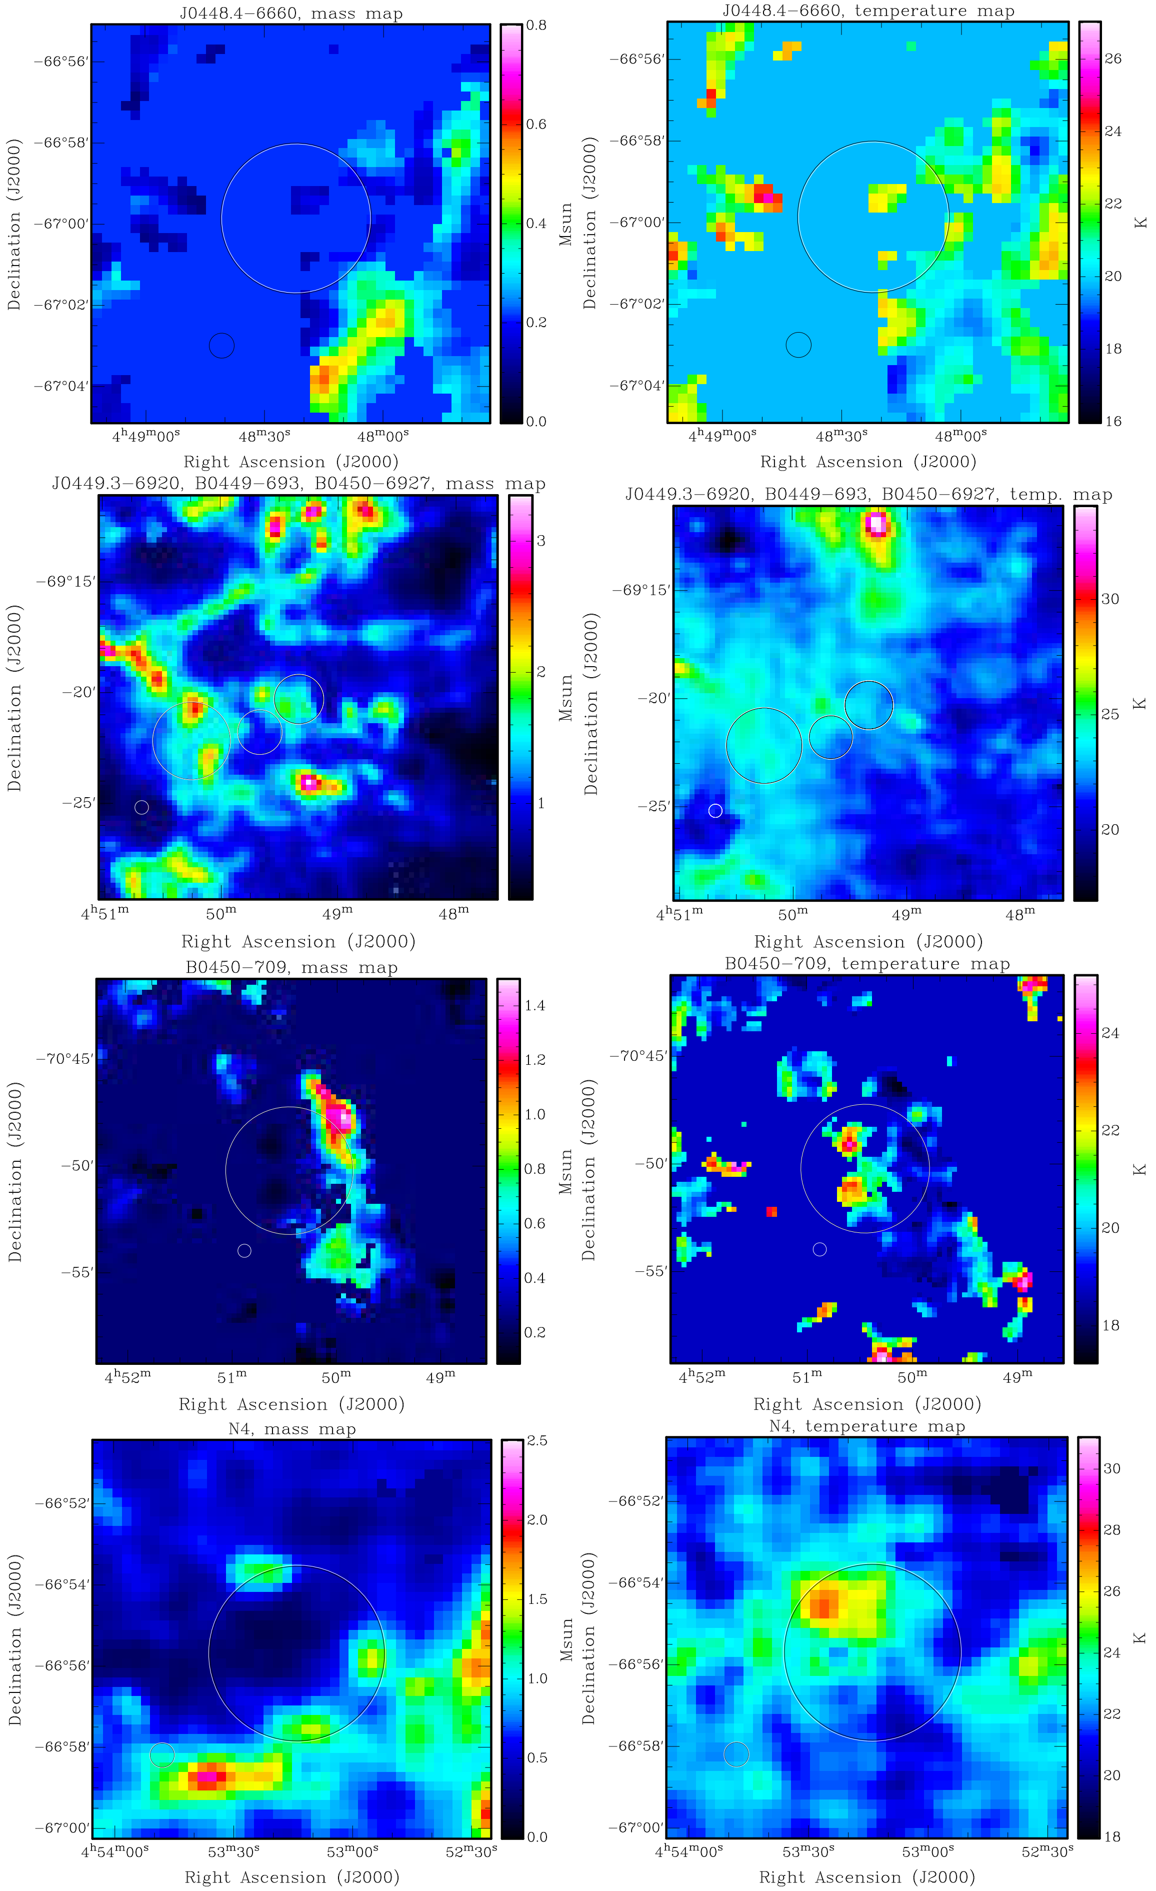


Fig. A.1.— *Left:* dust mass maps; *Right:* dust temperature maps. *a* and *b:* J04486658; *c* and *d:* J0449.3-6920 (center of the image), B0449-693 (circle in the middle) and B0450-6927 (on the left); *e* and *f:* B0450−70.9; *e* and *f:* N4.

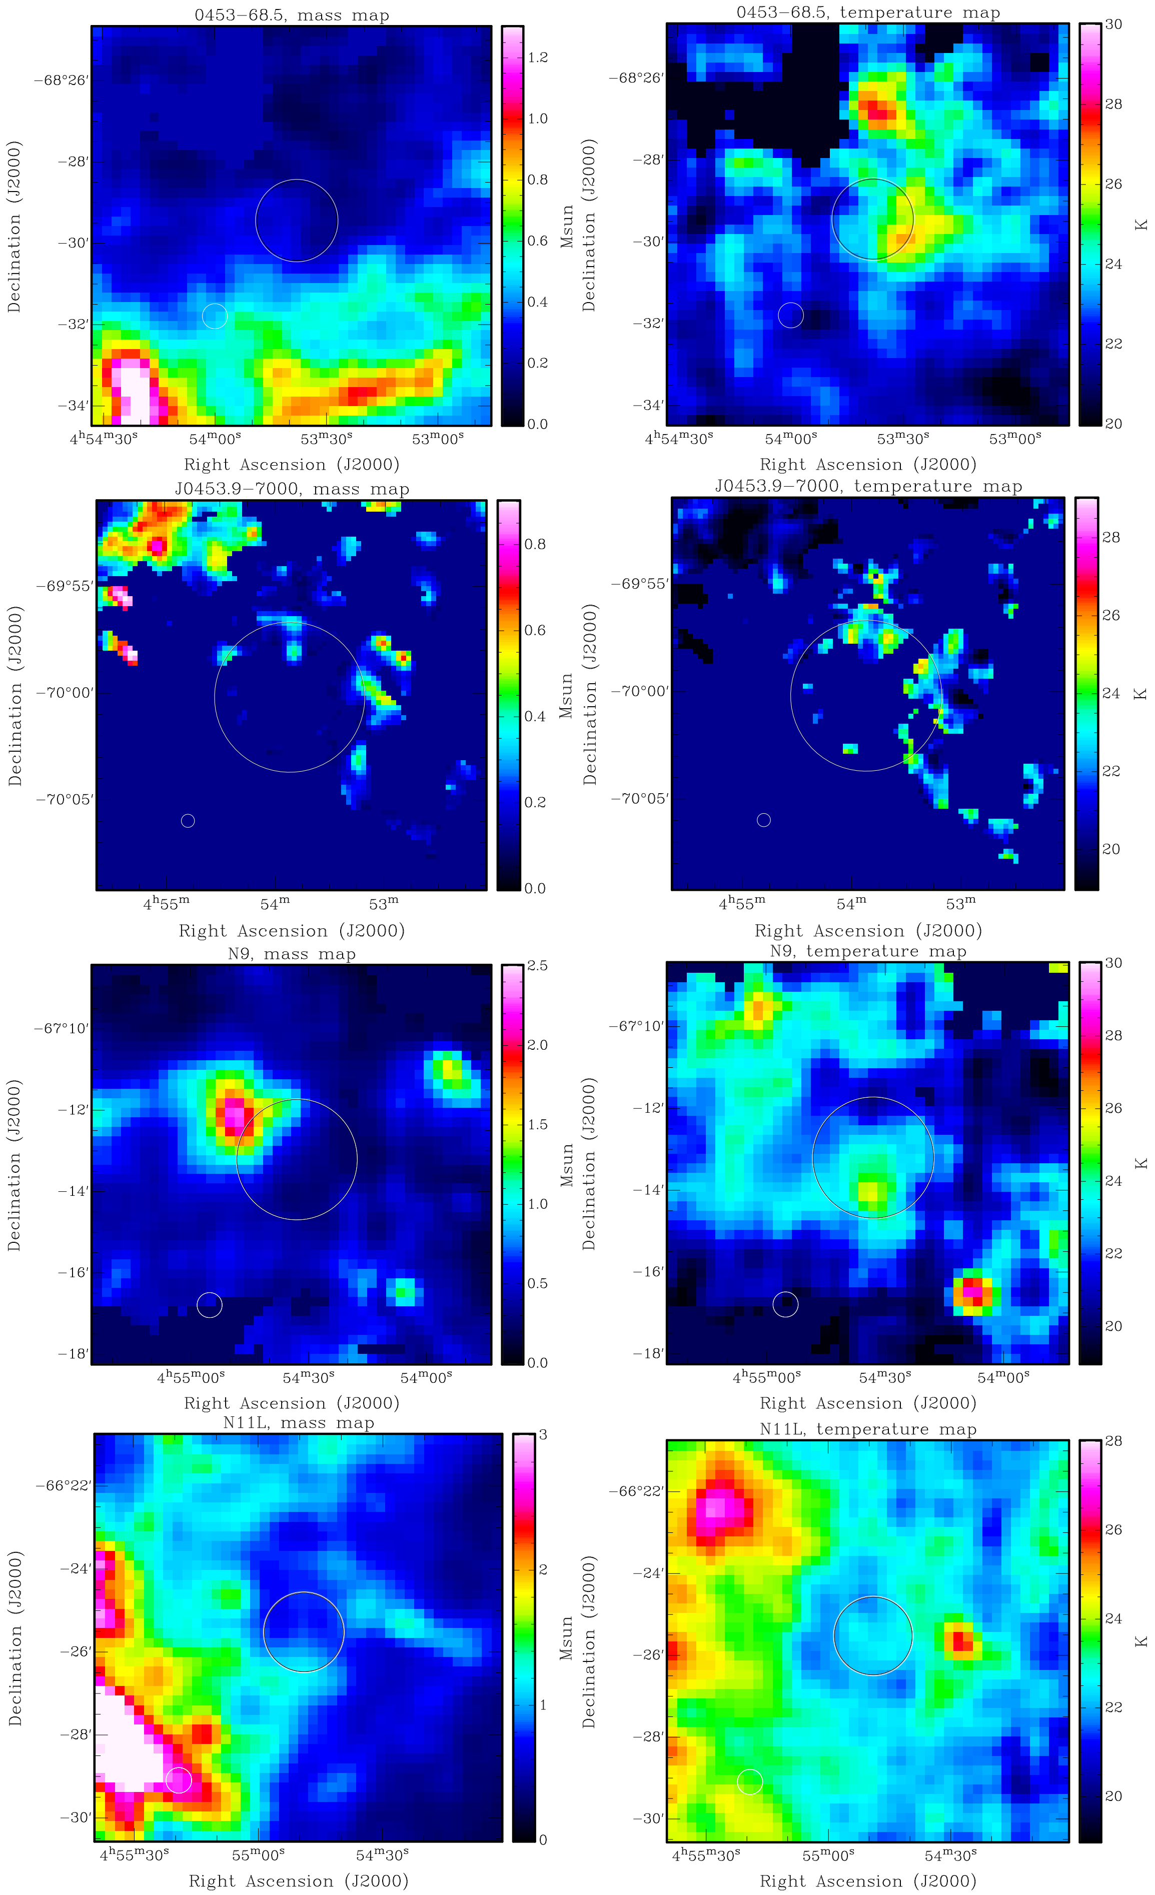


Fig. A.2.— SNR 0453−68.5, and SNR J0453.9−7000, SNR N 9, and SNR N 11L.

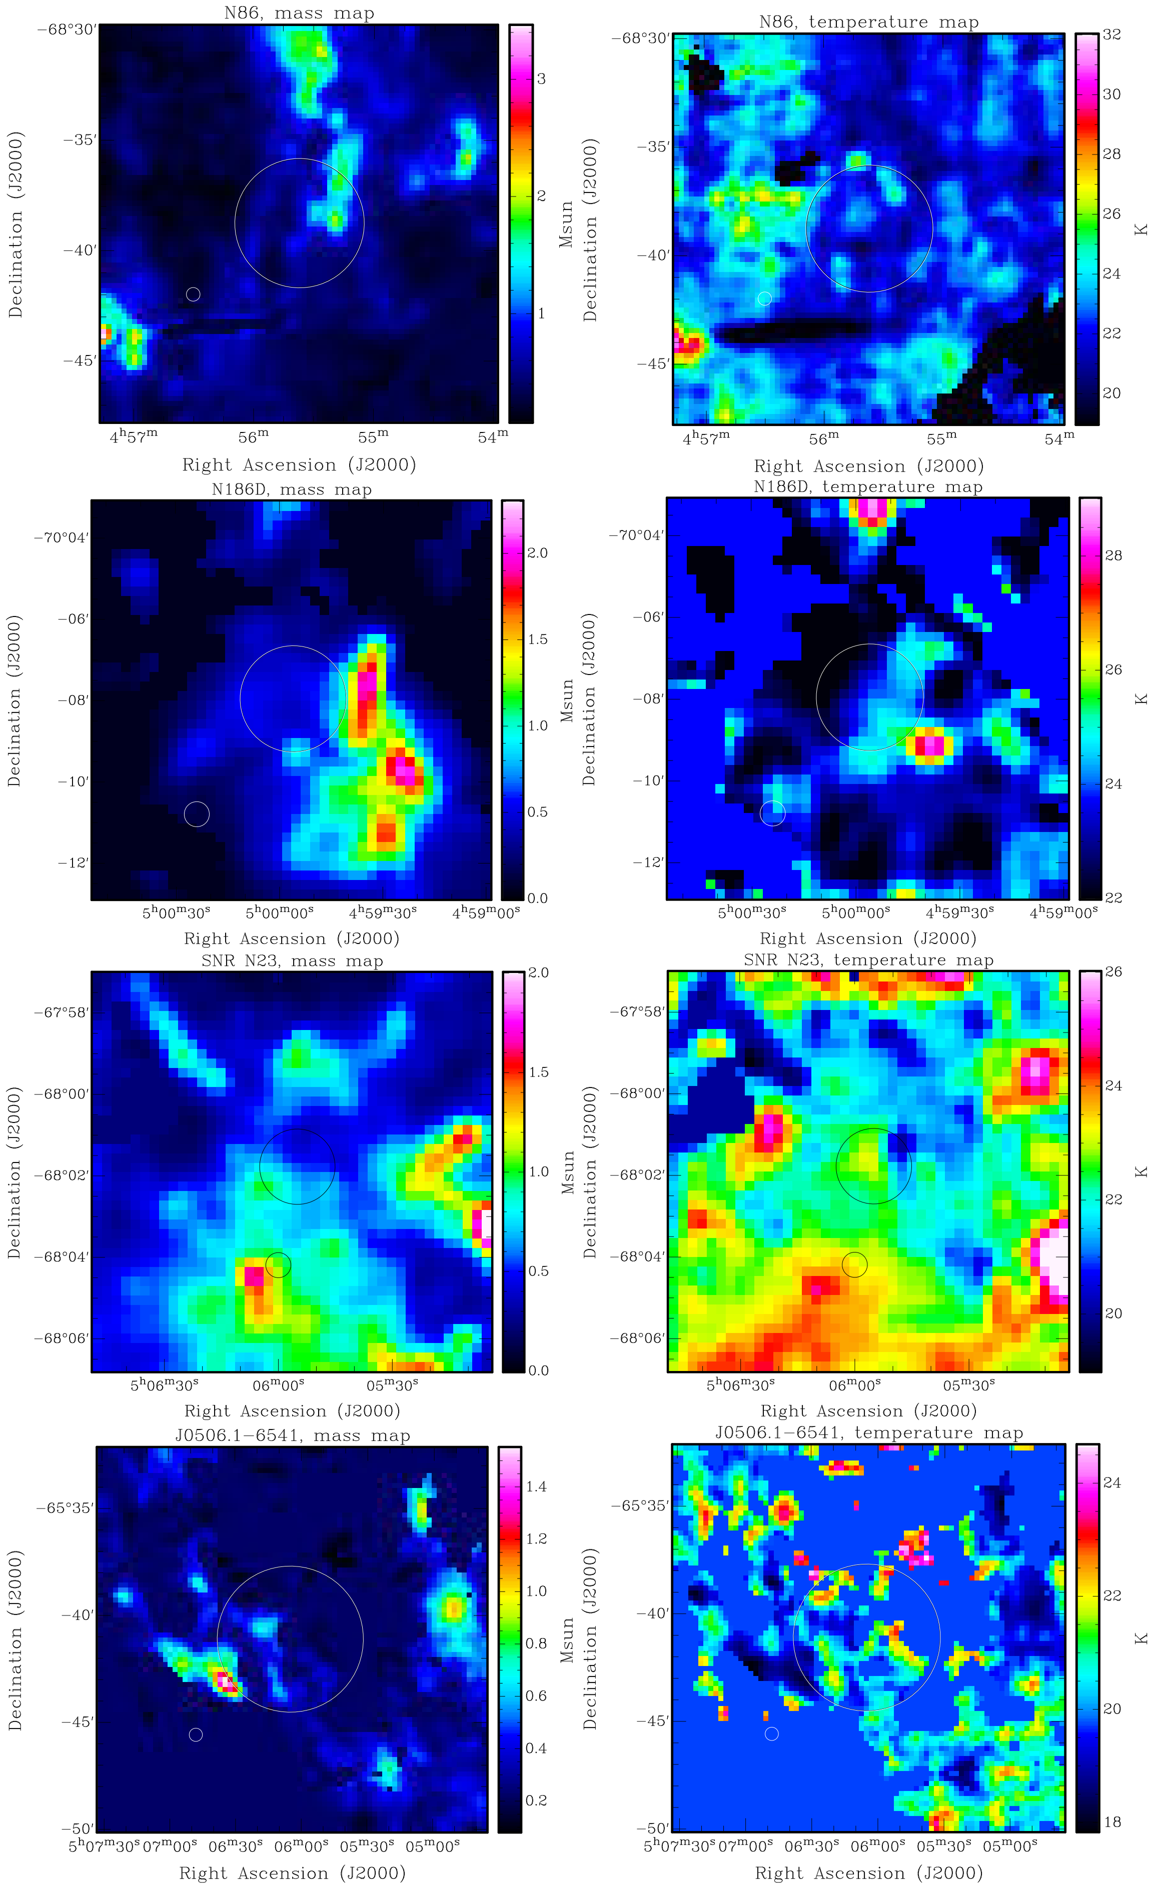


FIG. A.3.— SNR N 86, N 186D, N 23 and J 05066541.

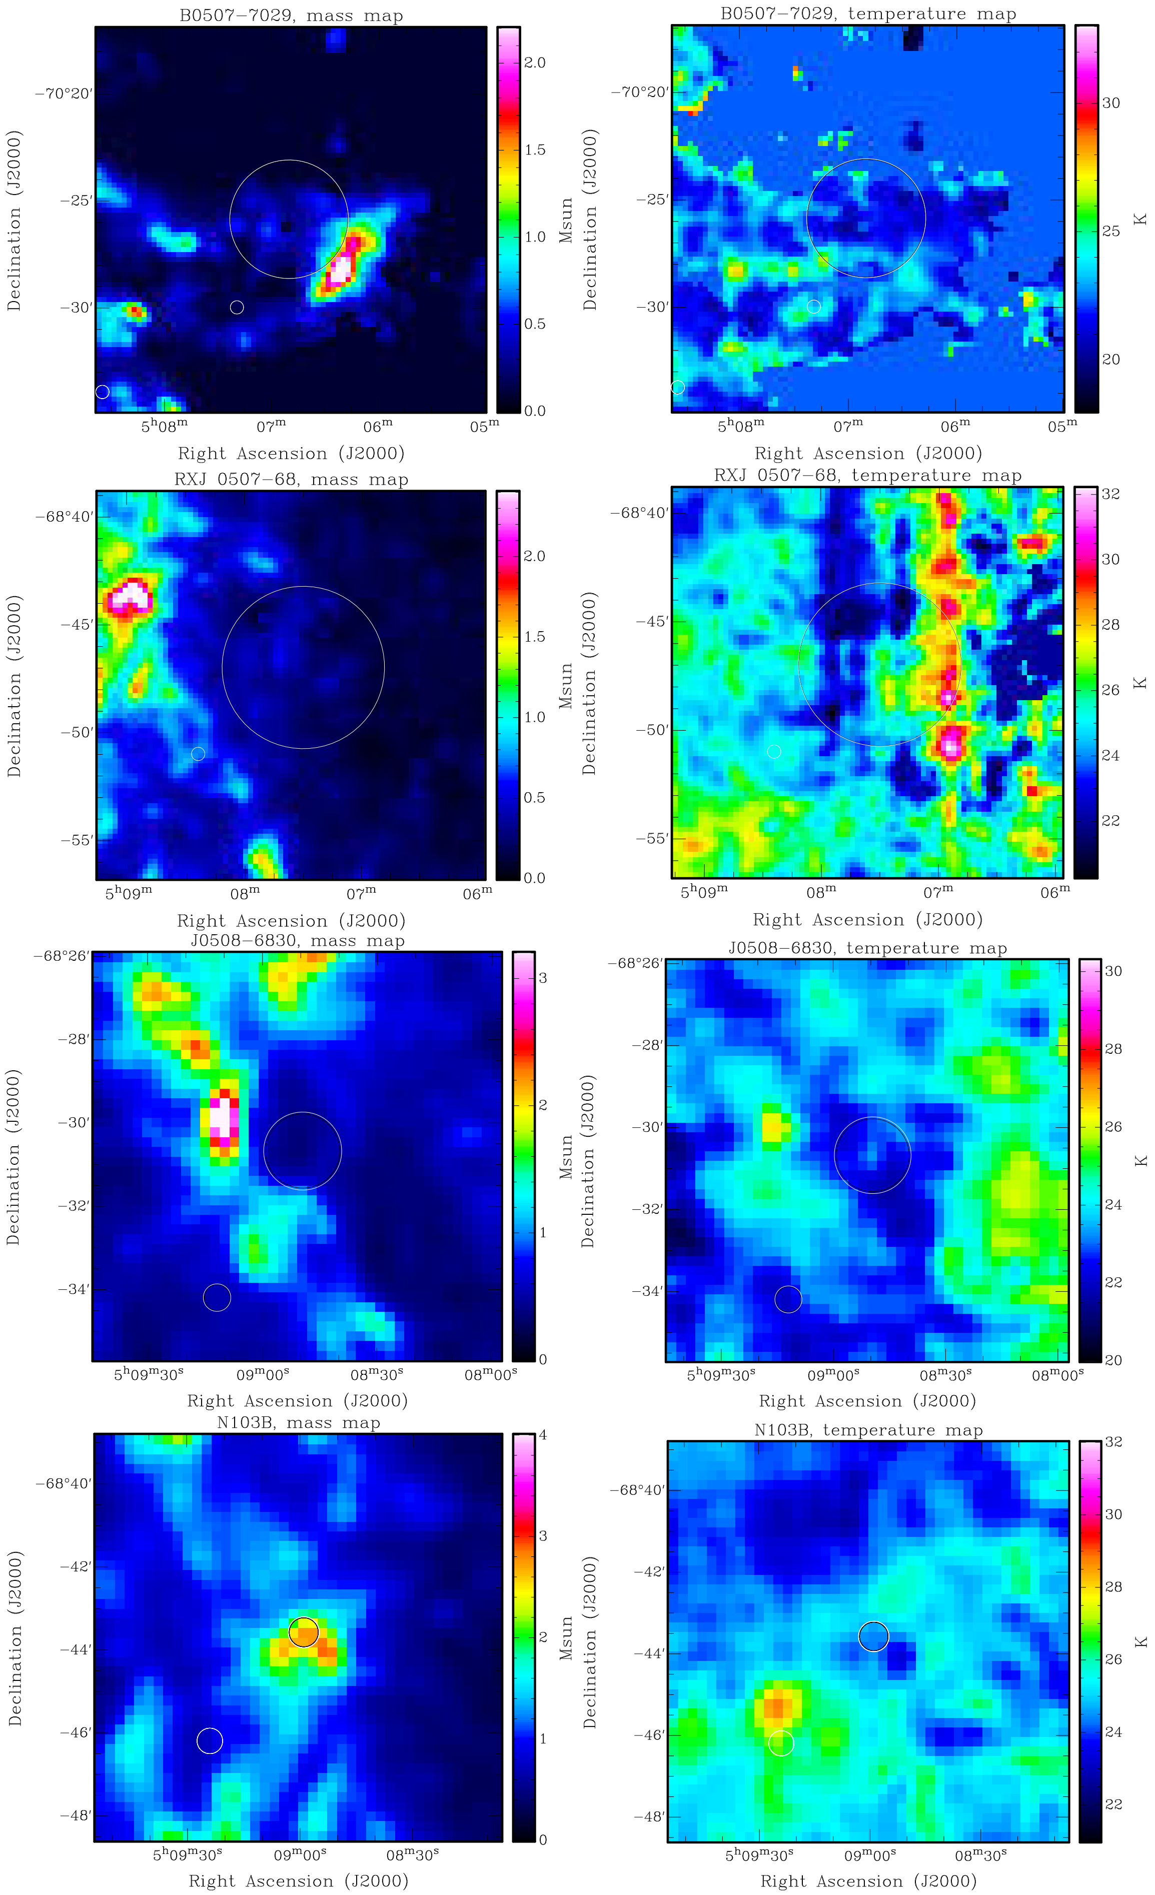


FIG. A.4.— SNR B 0507−7029, SNR RXJ0507−68, J 0508-6830 and N 103B.

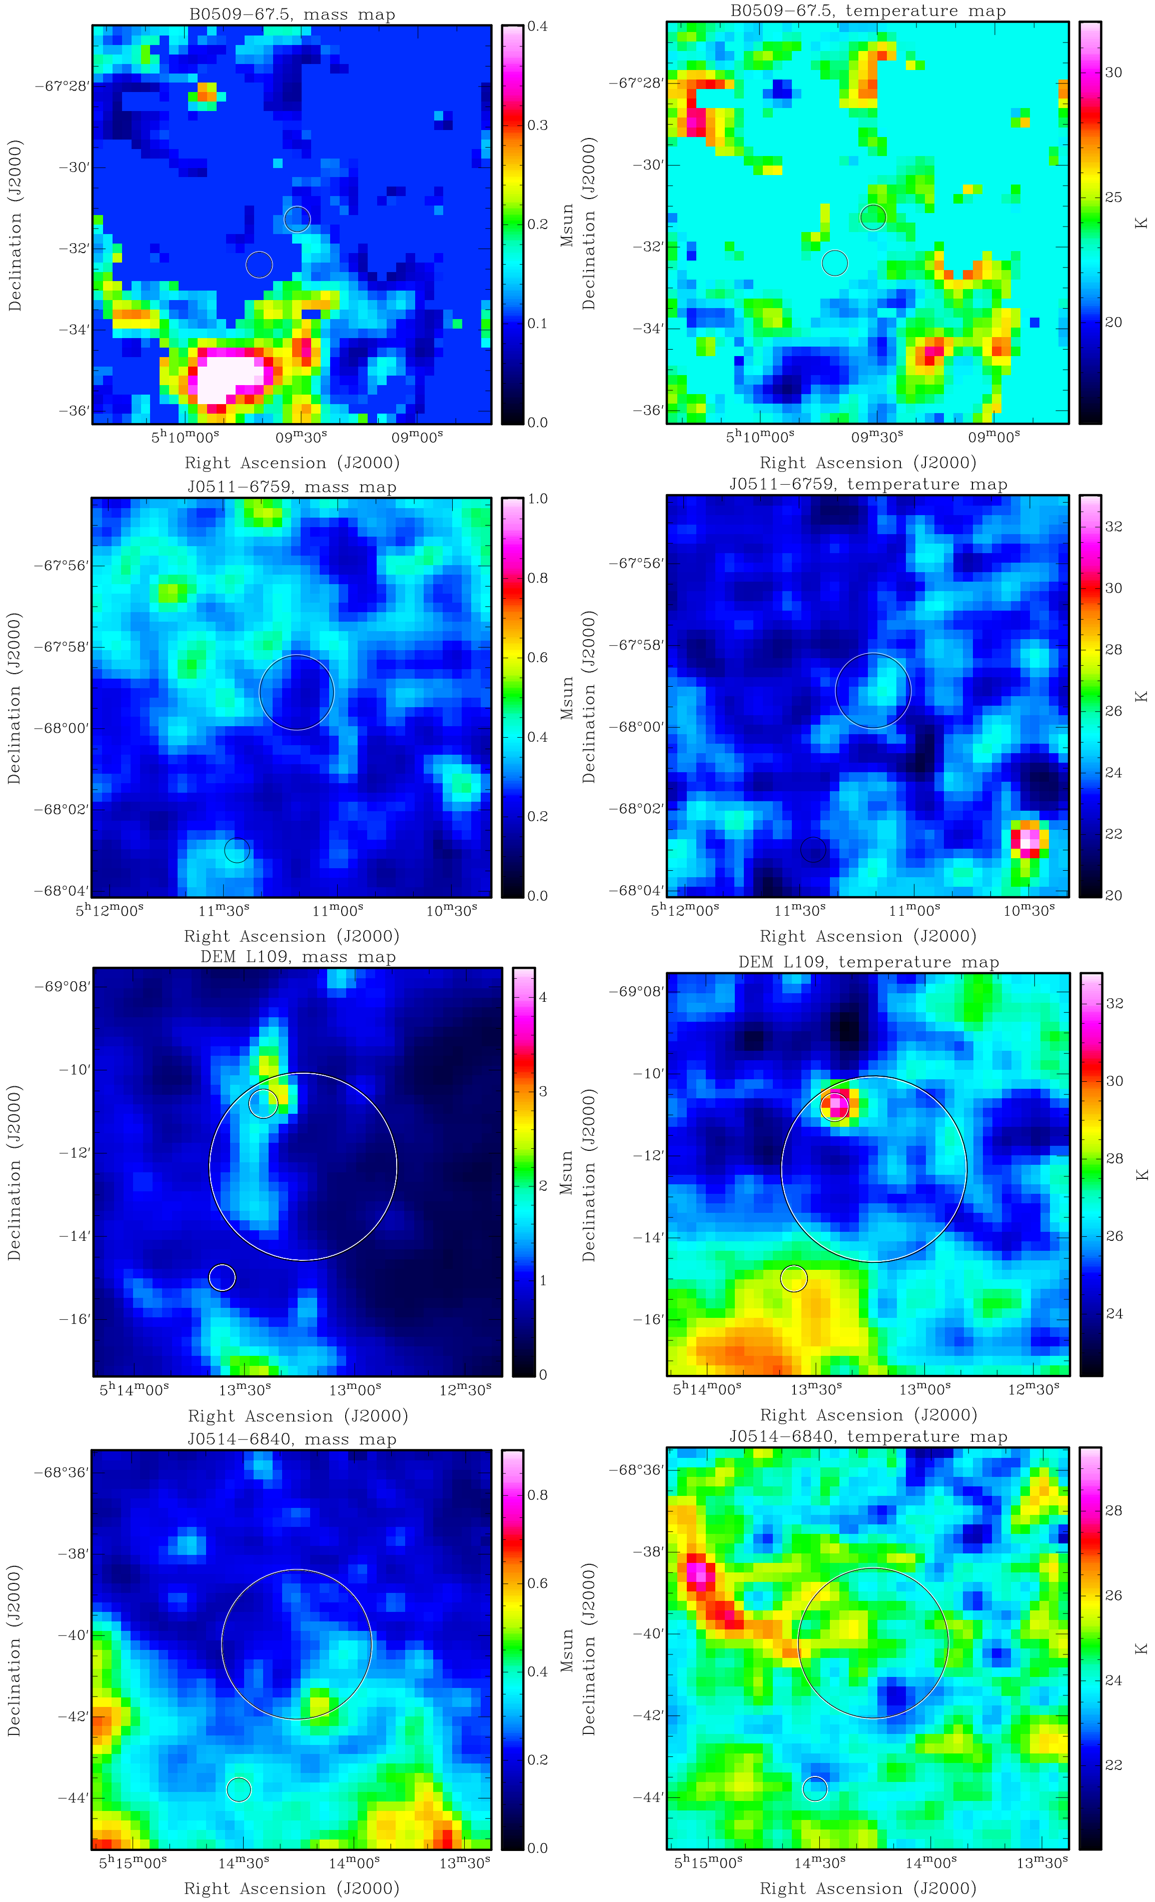


FIG. A.5.— SNR B 0509-67.5, J 0511-6759, DEM L109 (and the small candidate inside; Bojicic et al. 2007) and J 0514−6840.

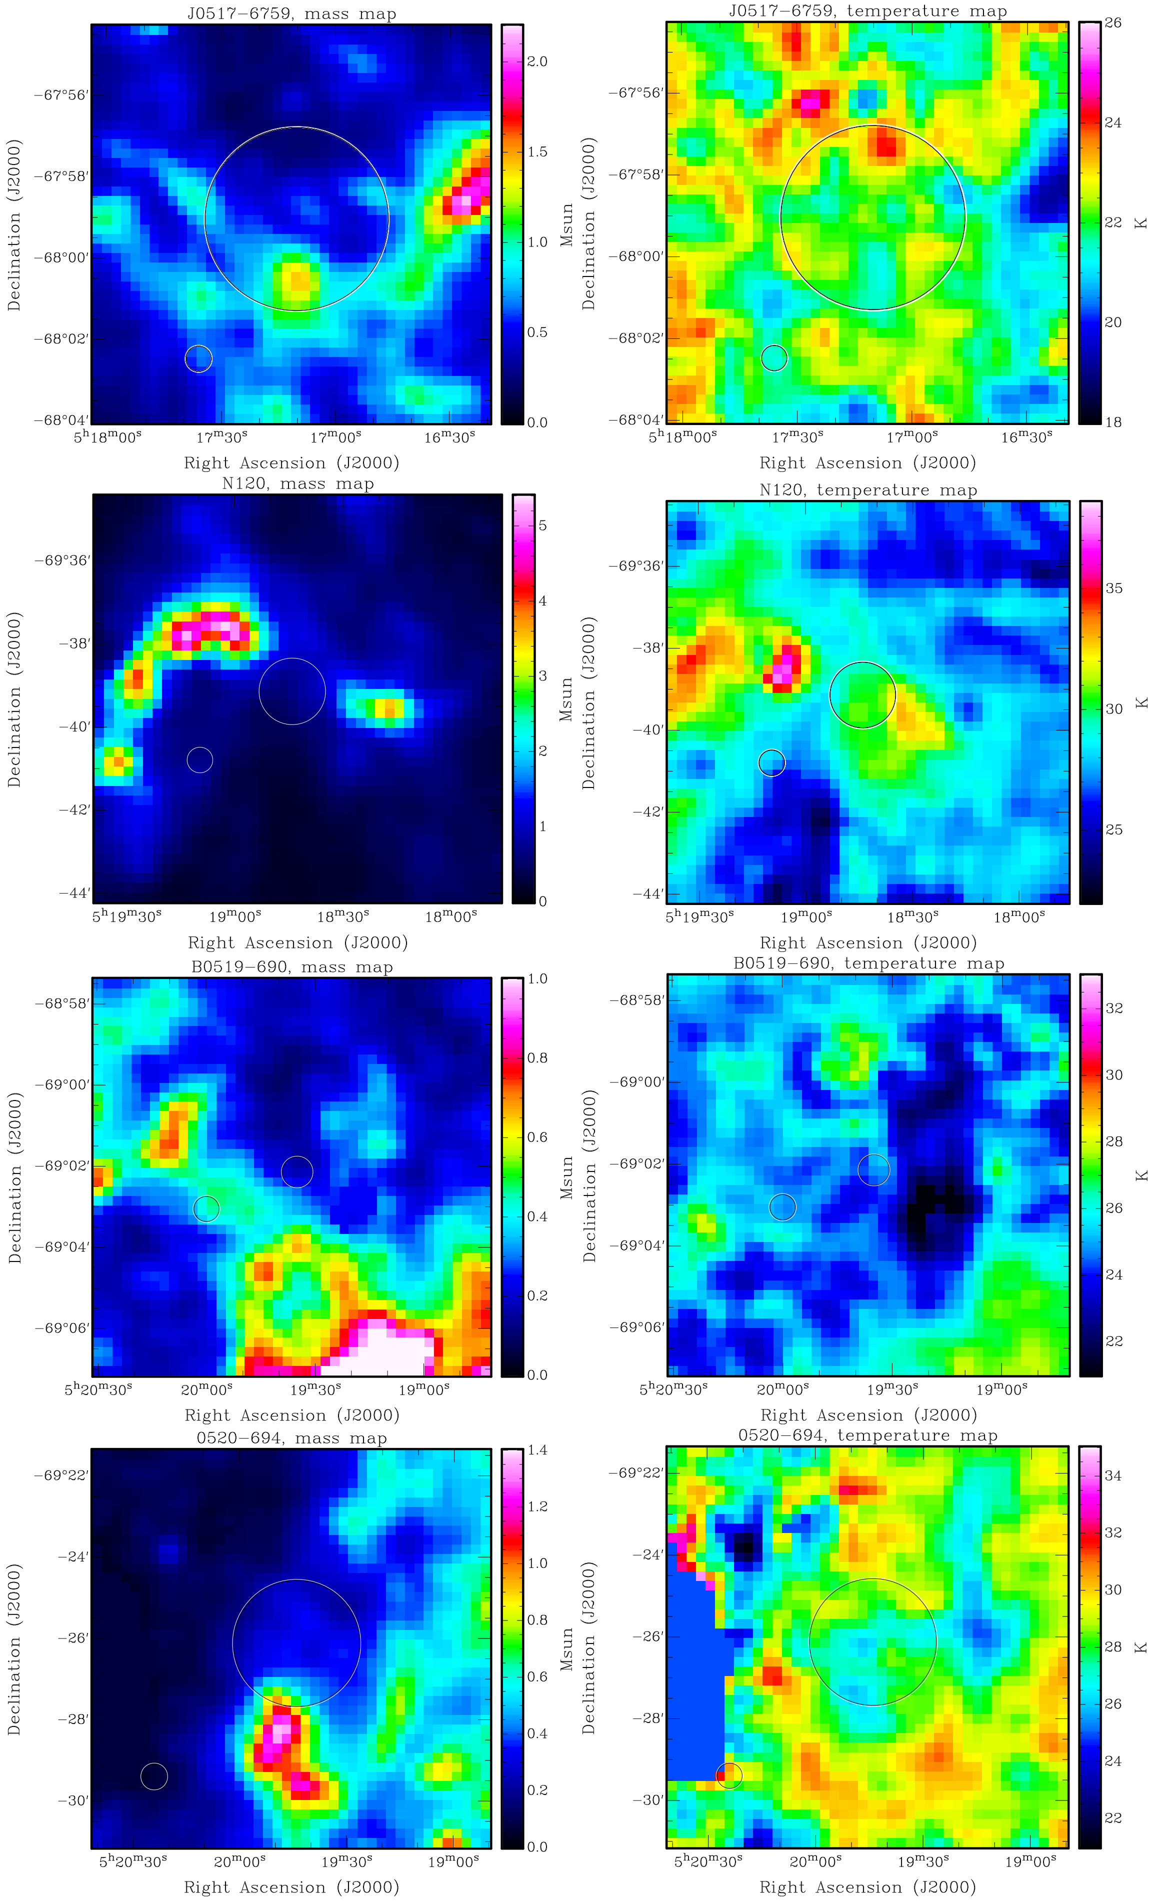


FIG. A.6.— SNR J 0517-6759, N120, B 0519−690 and 0520−69.4.

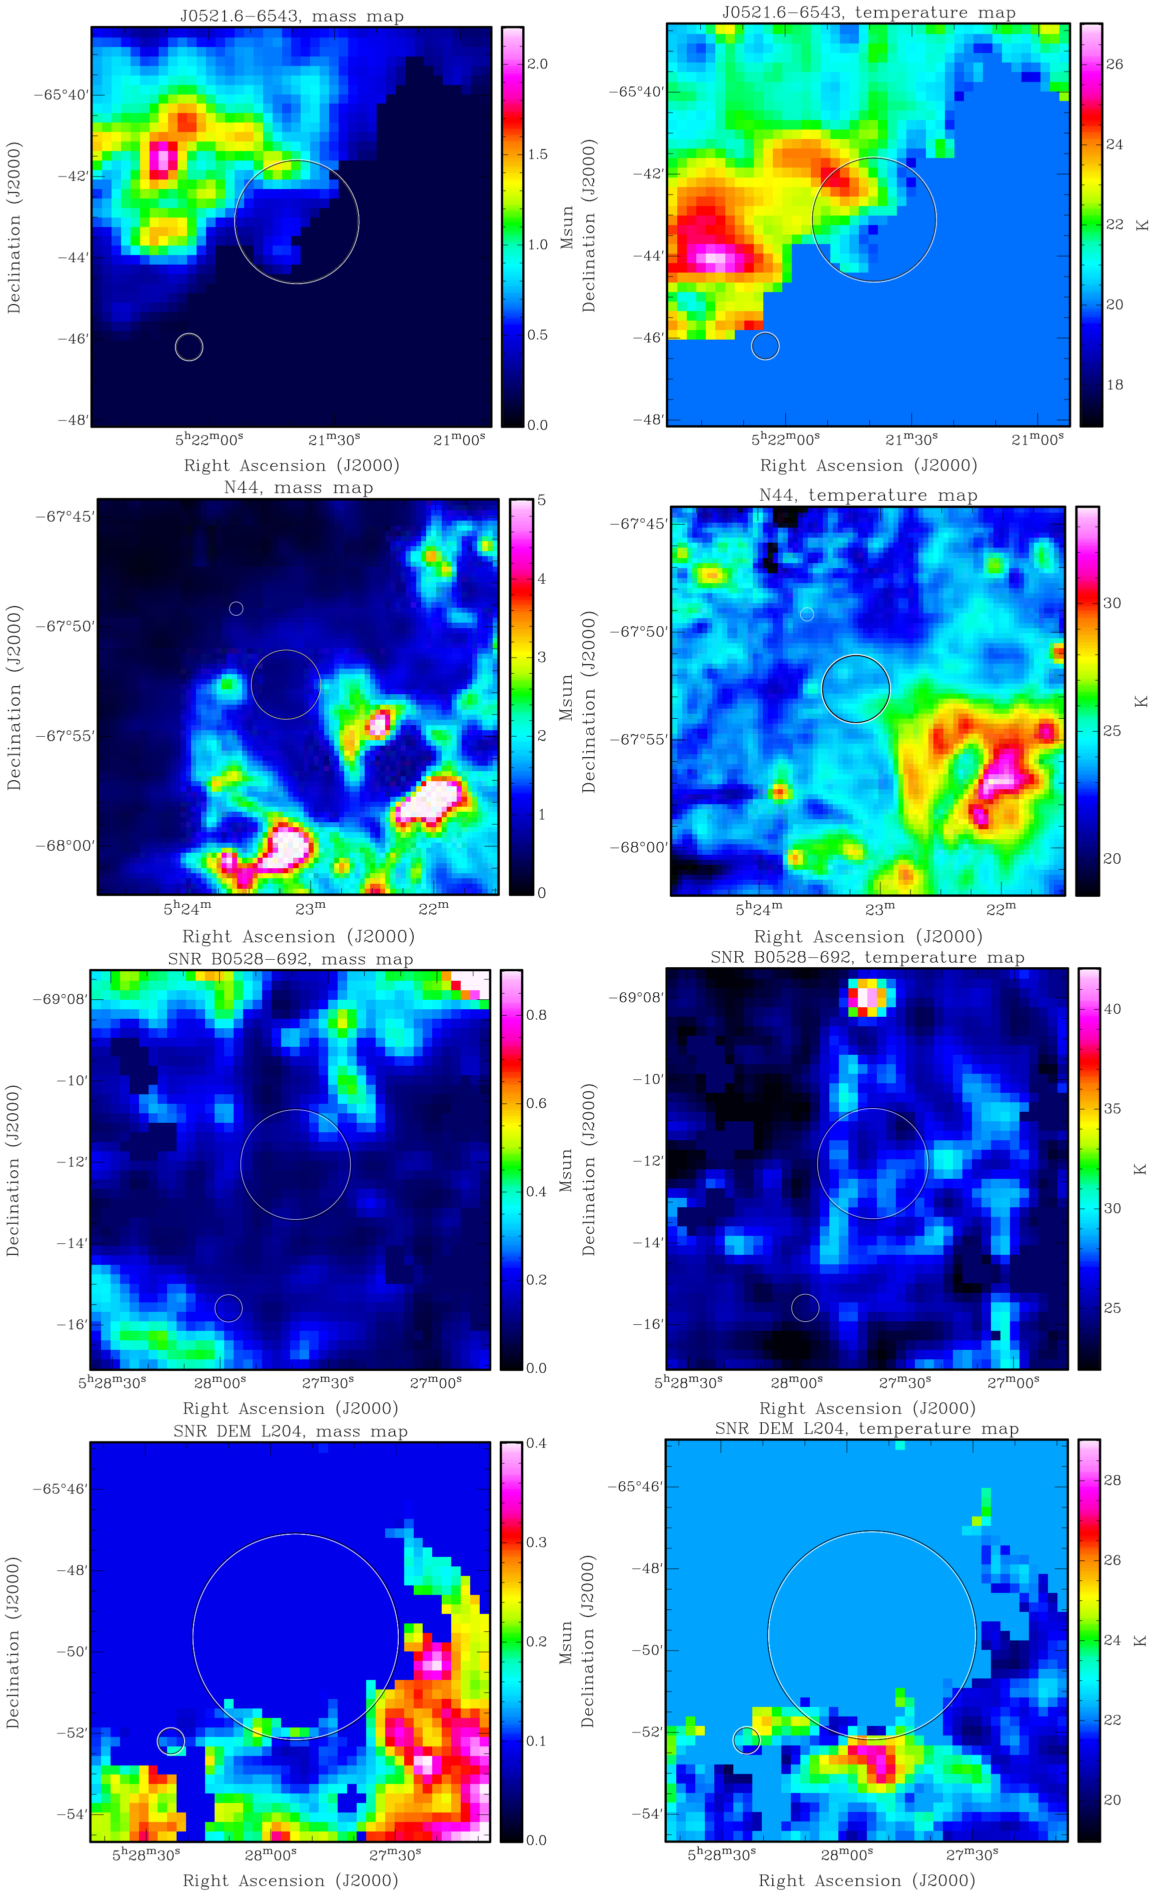


FIG. A.7.— J 0521.6−6543, N44, 0528−692 and DEM L204.

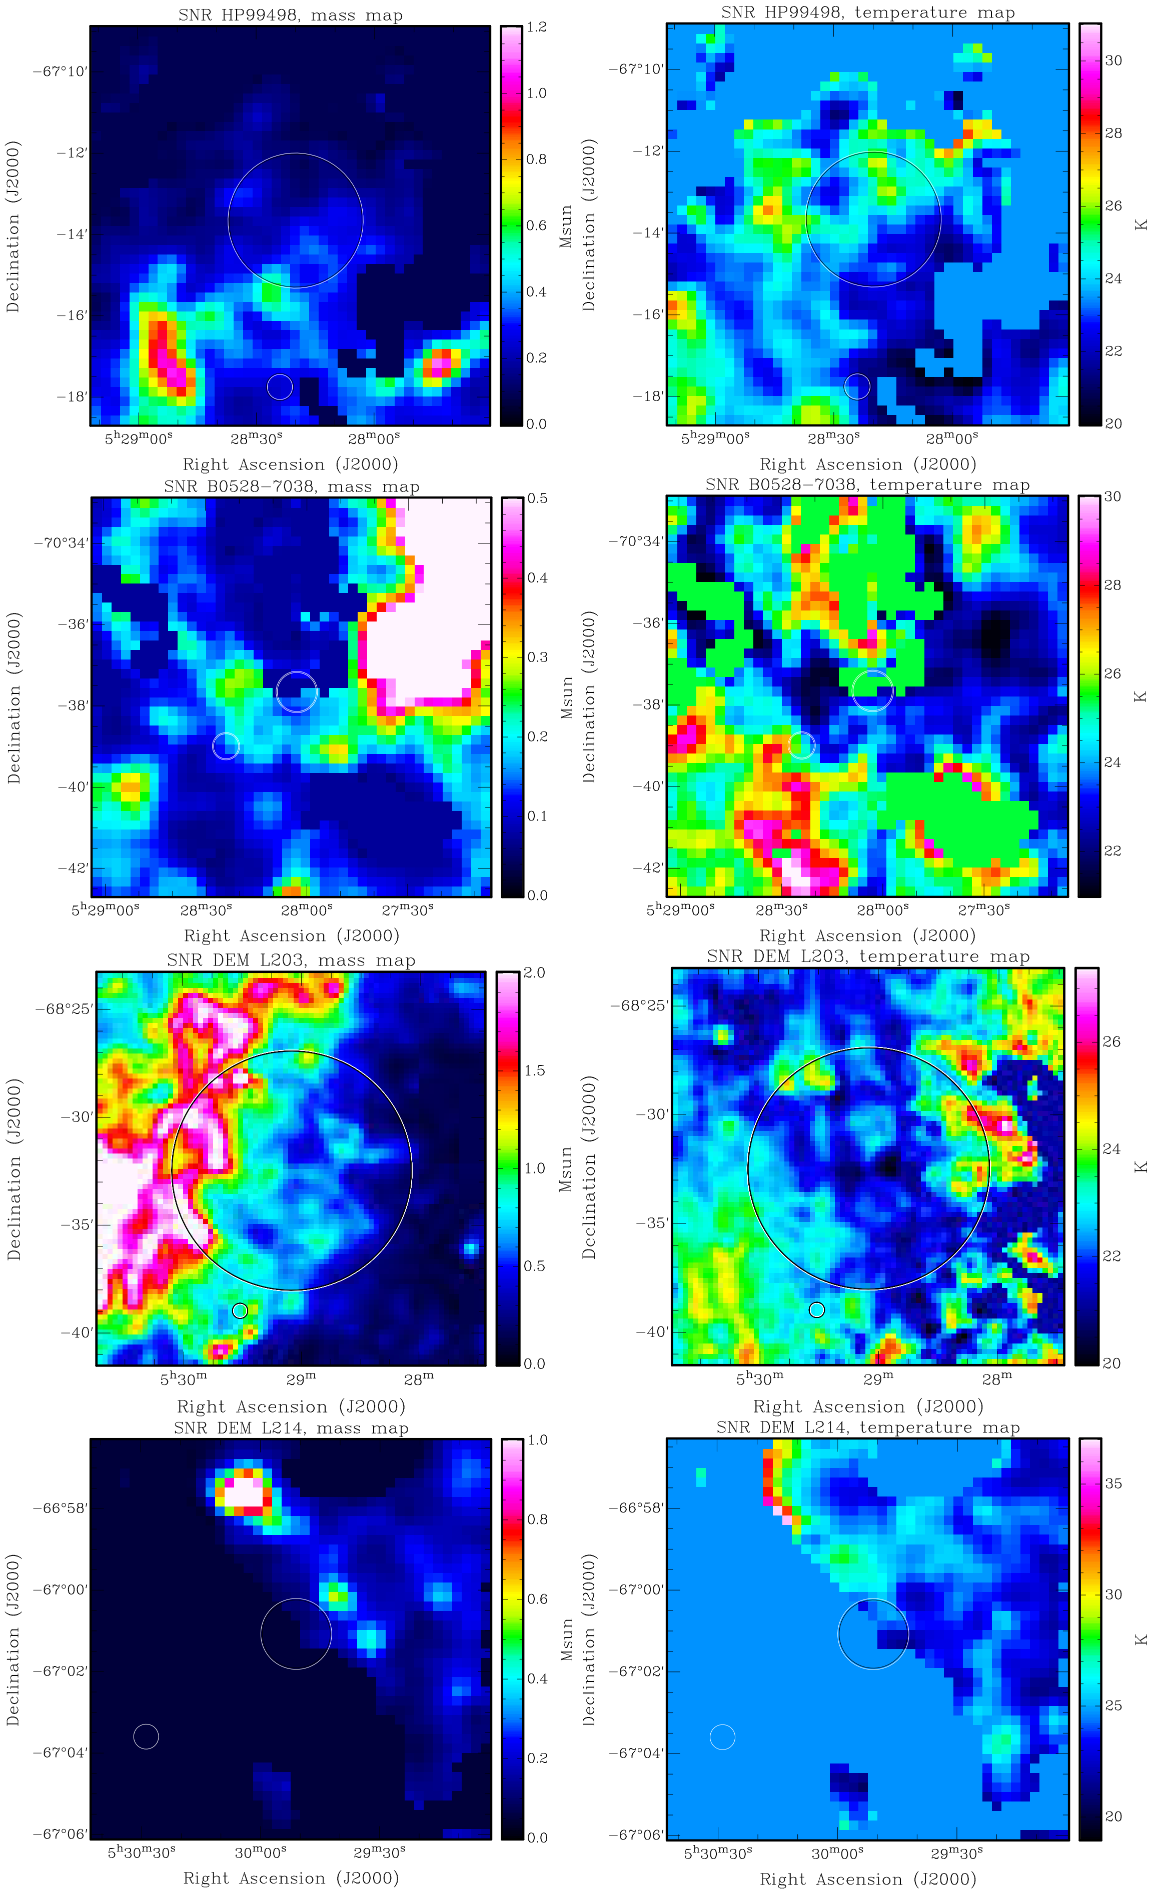


FIG. A.8.— SNR HP99498, B 0528-7038, DEM L203 and DEM L214 from Badenes et al. 2010.

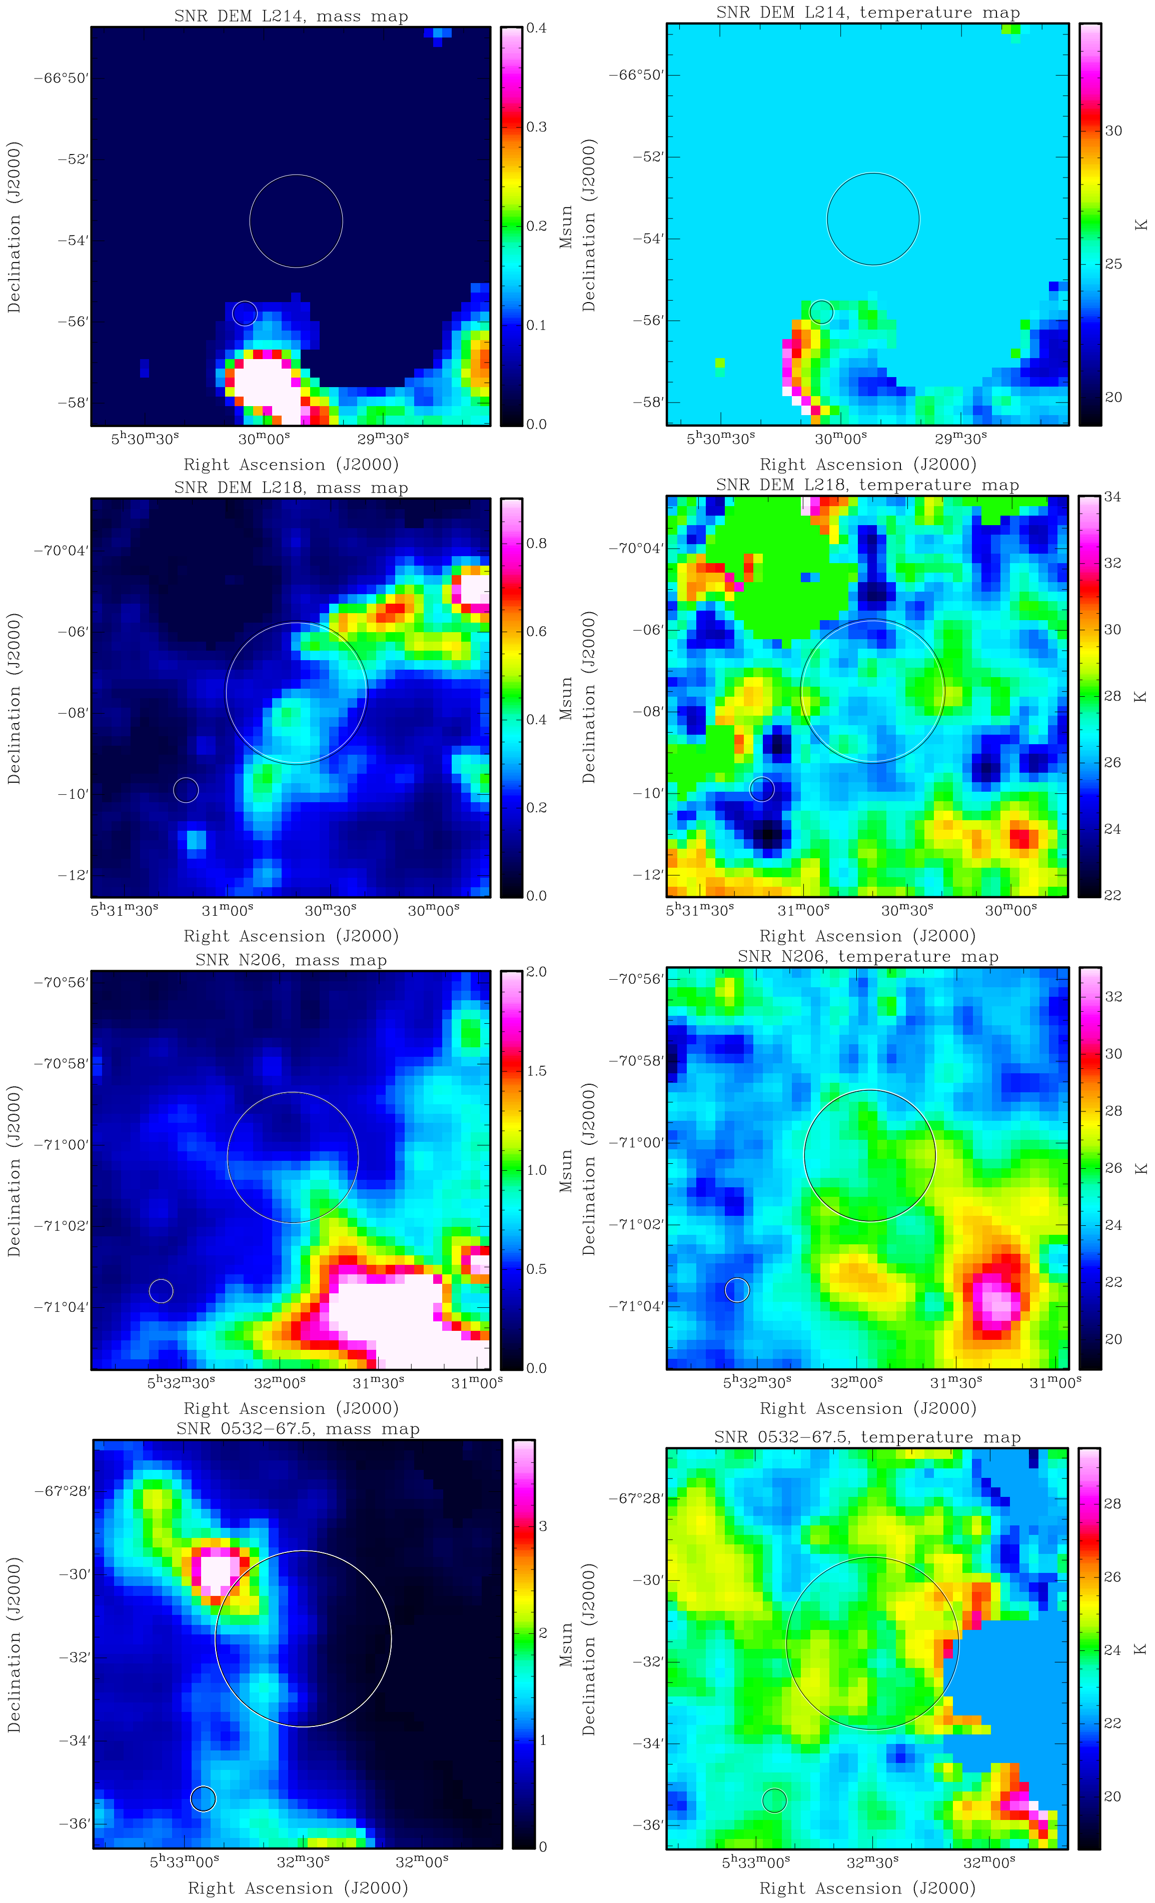


FIG. A.9.— SNR DEM L214 (Bozzetto et al. 2011), DEM L218. N 206 and 0532−67.5.

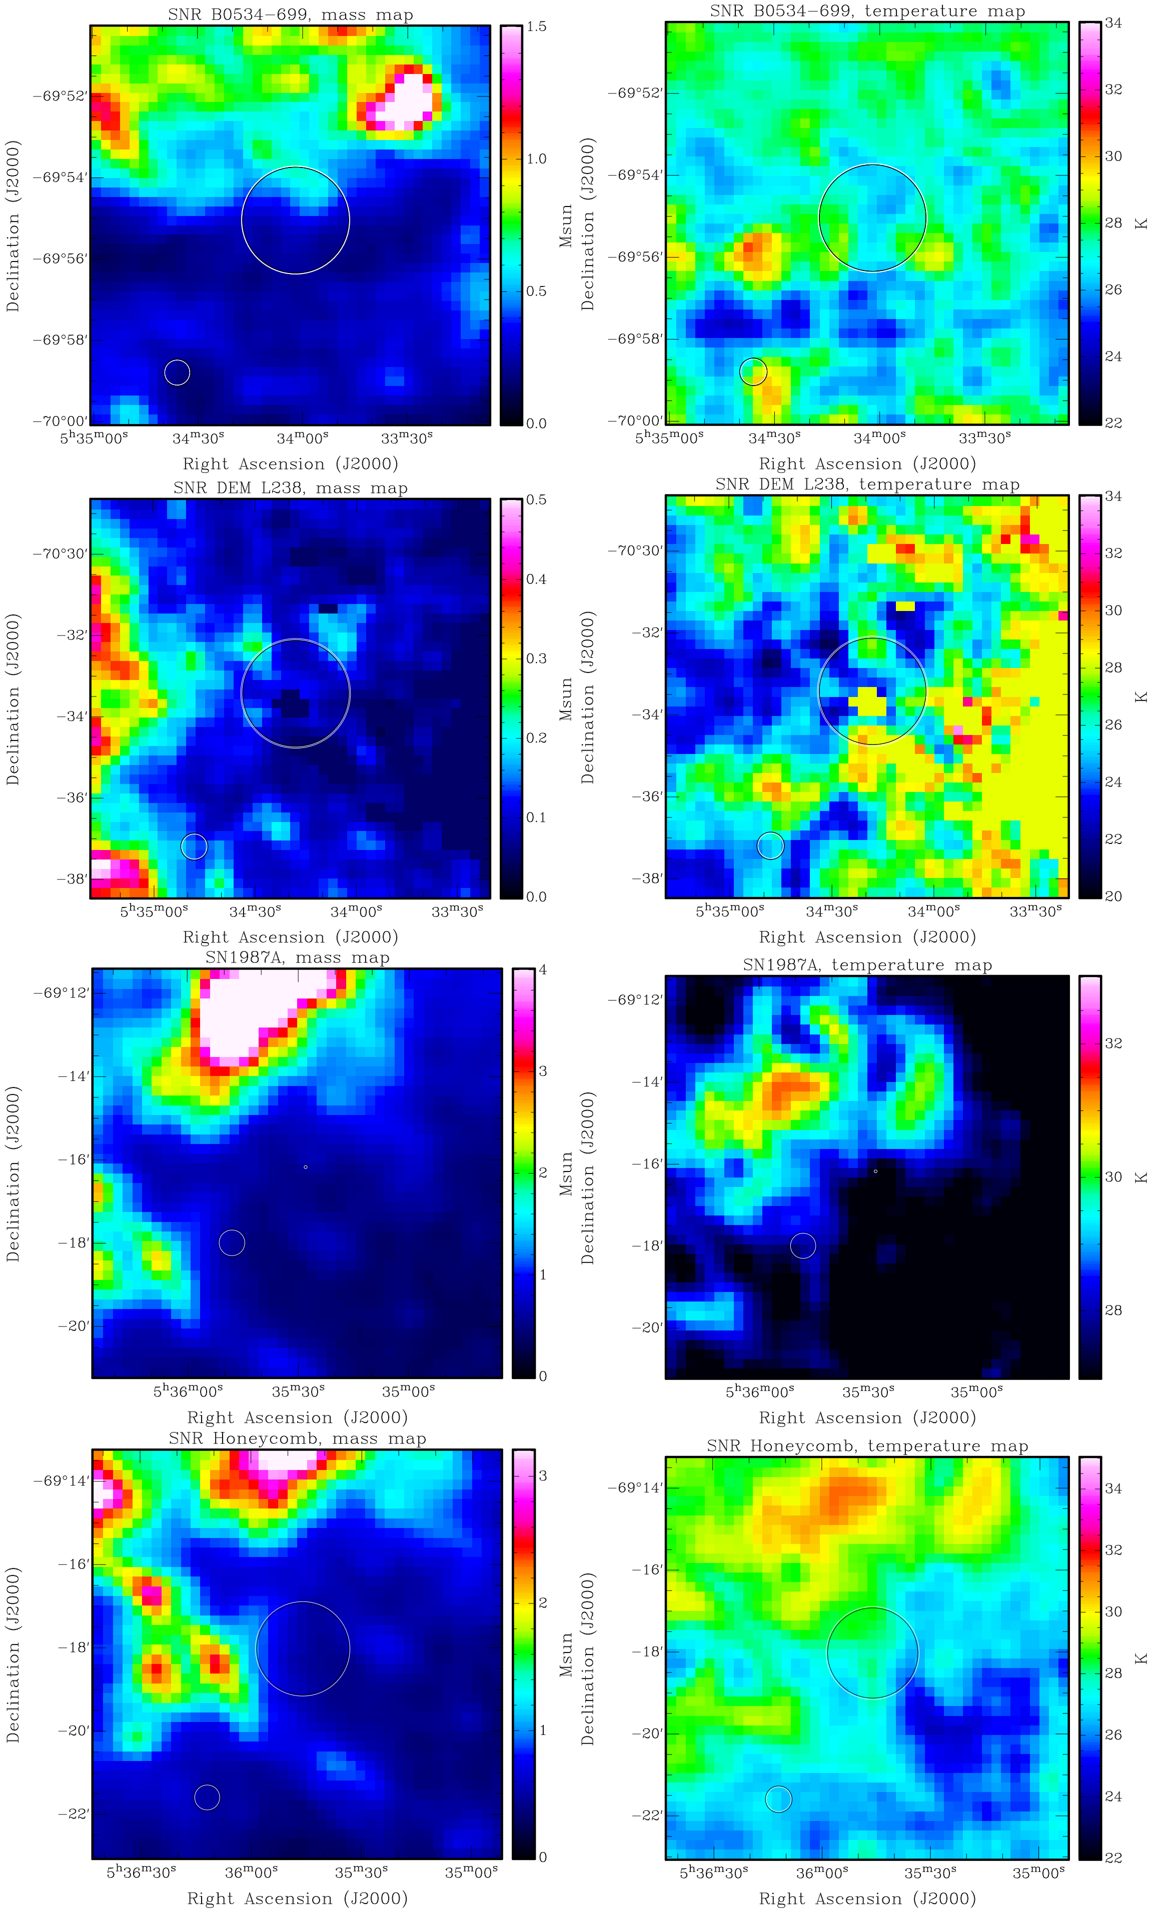


FIG. A.10.— B 0534-699, DEM L238, SN 1987A and SNR Honeycomb.

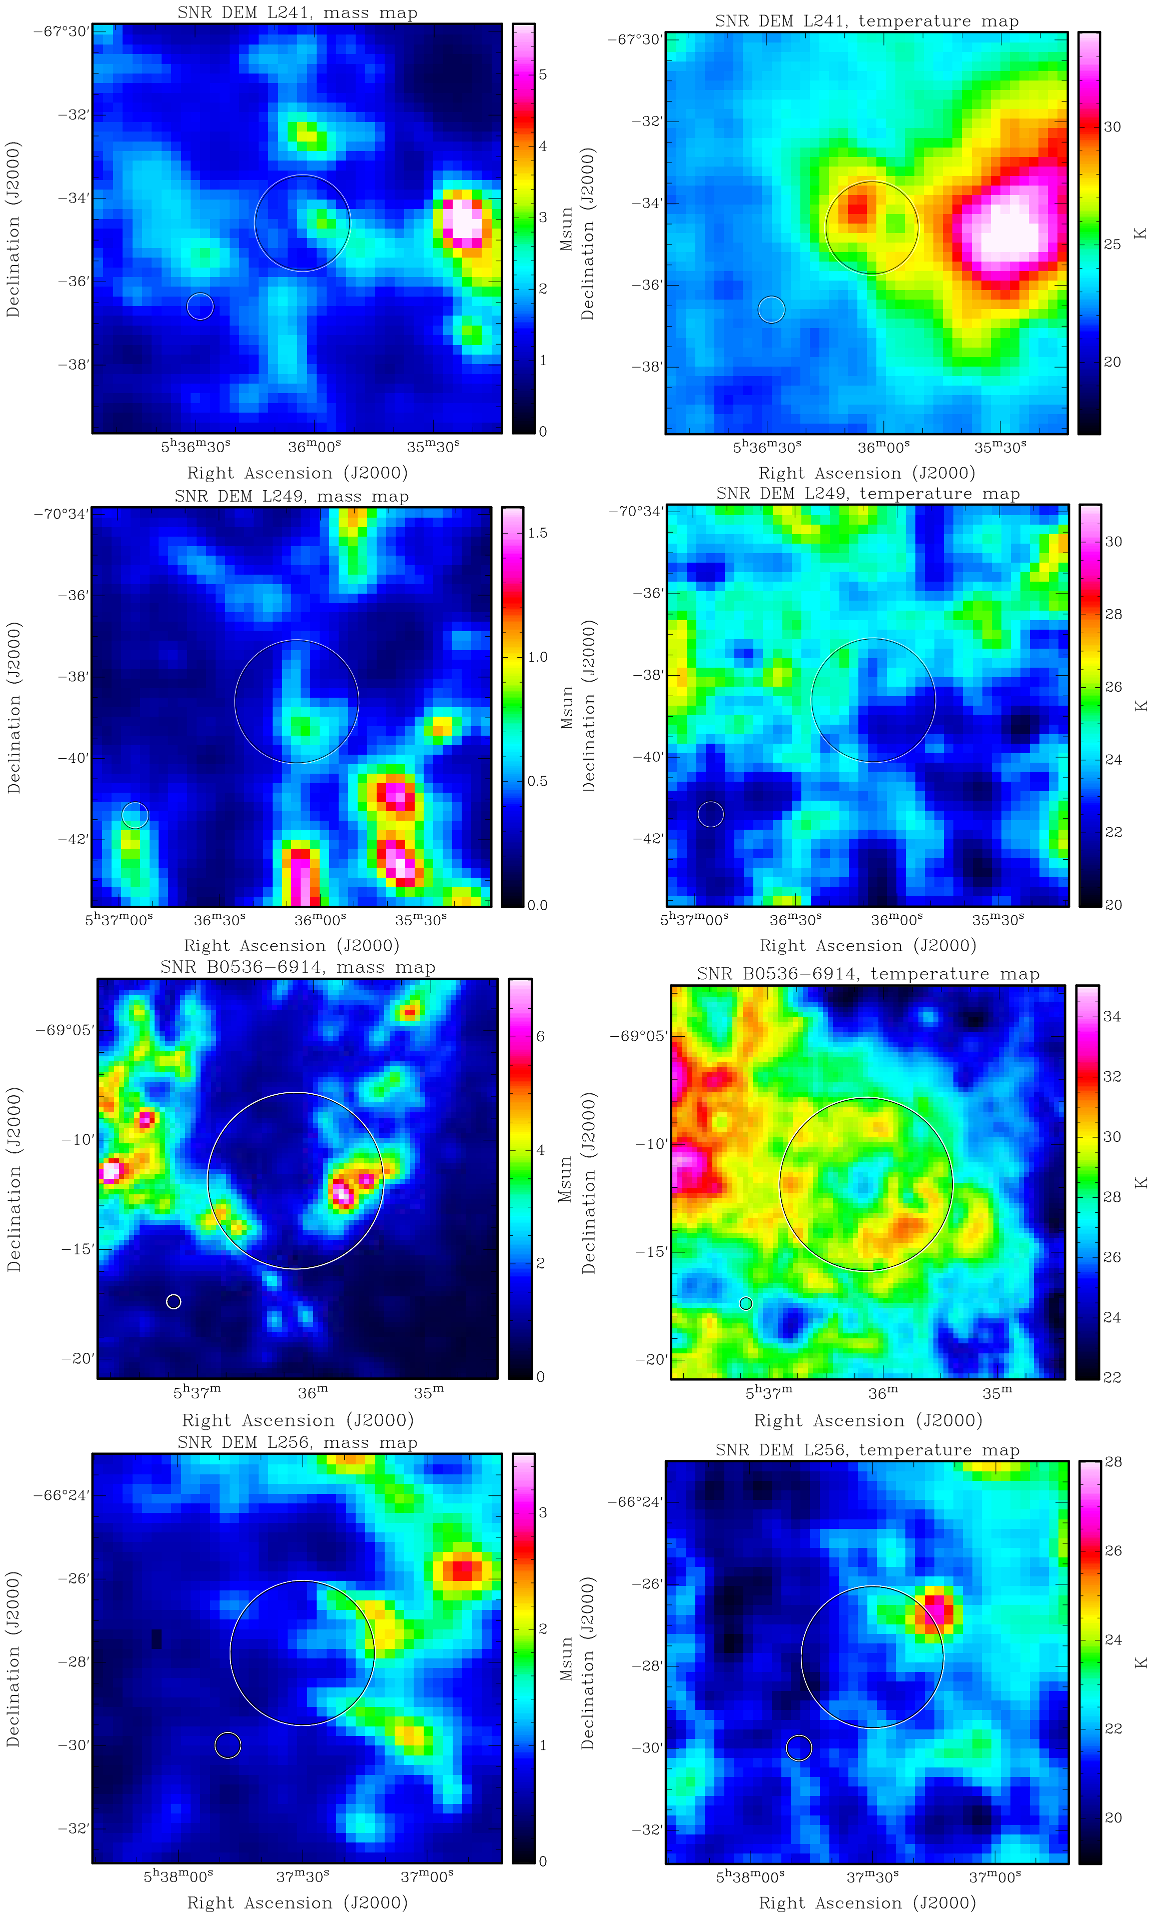


FIG. A.11.— DEM L241, and SNR DEM L249, SNR B 0536−6914 and SNR DEM L256.

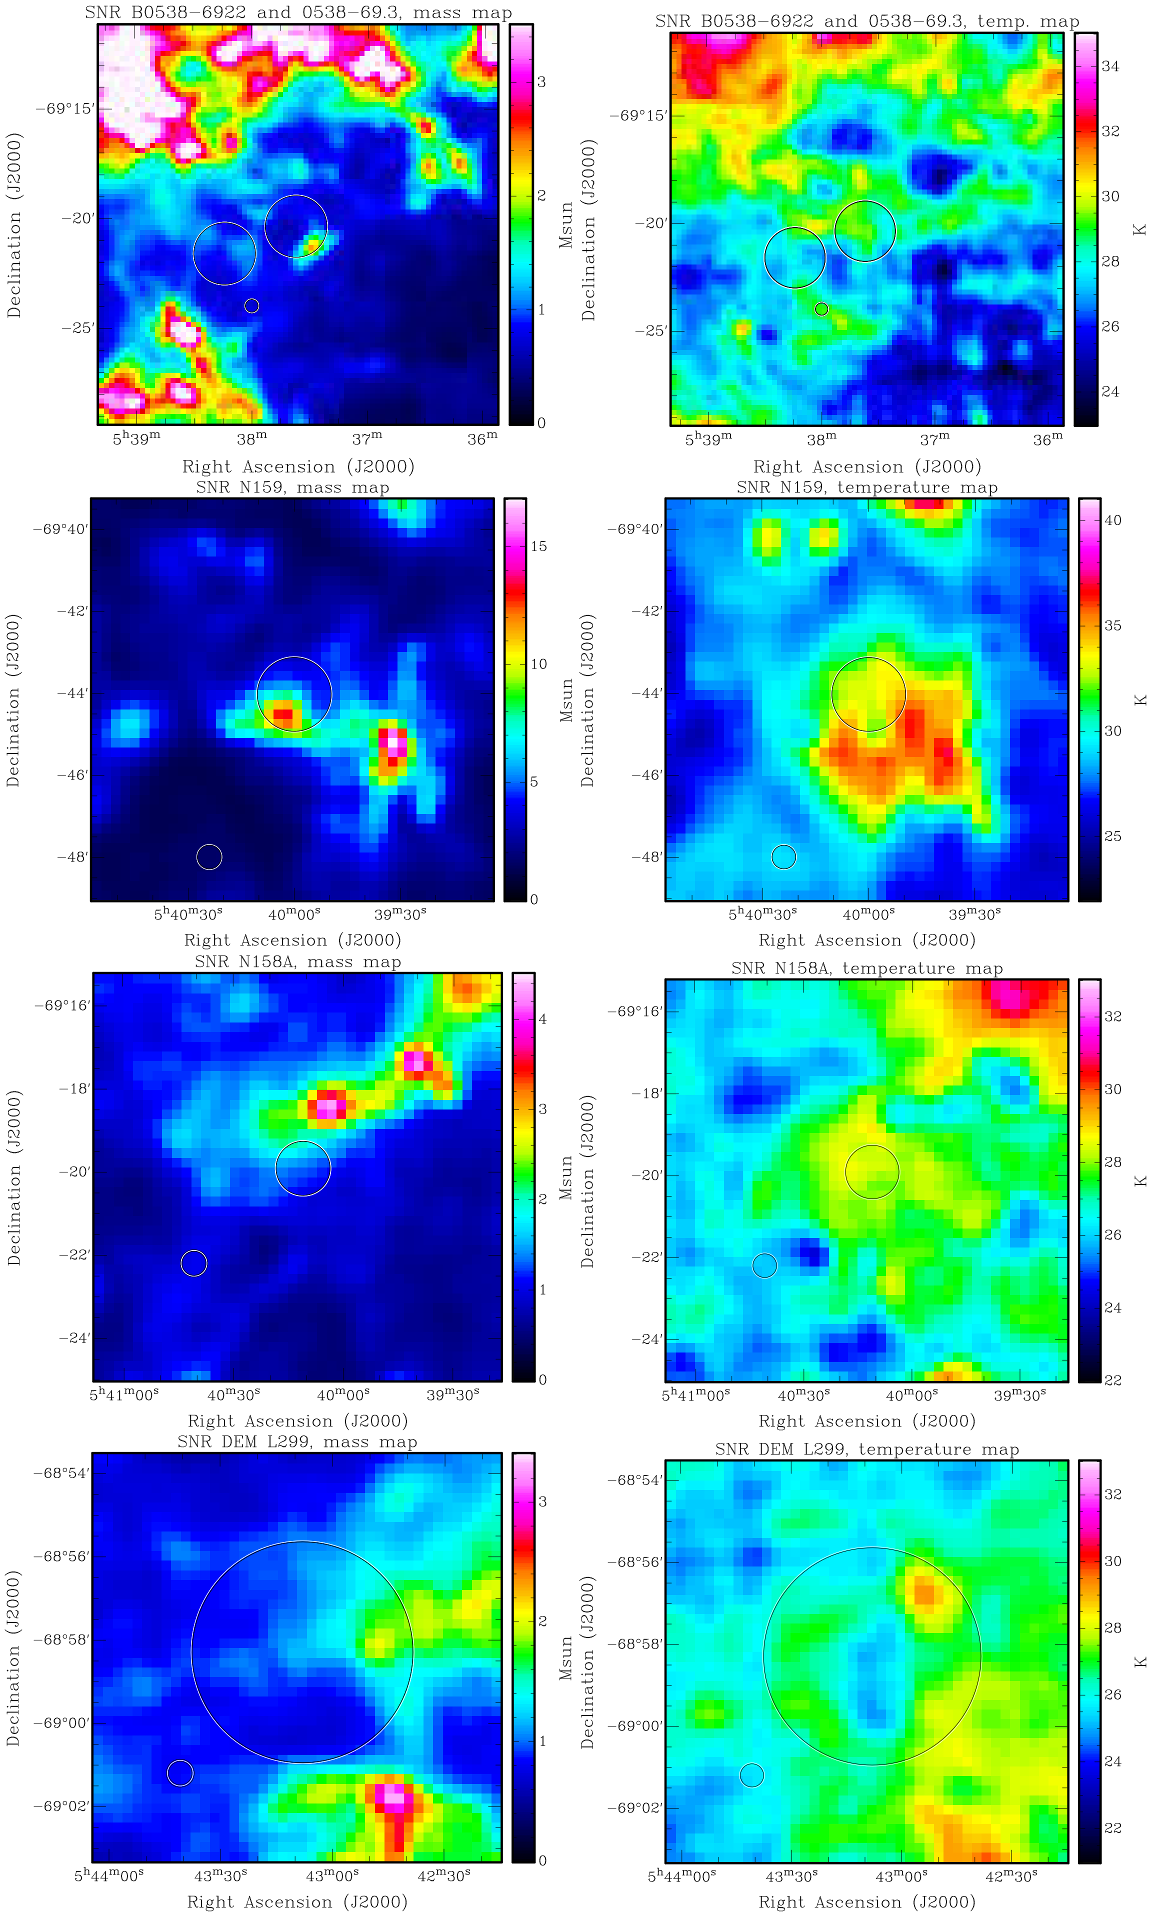


FIG. A.12.— B 0538−6922 (center) and 0538−693 (the second circle), N 159, N158 A and DEM L299.

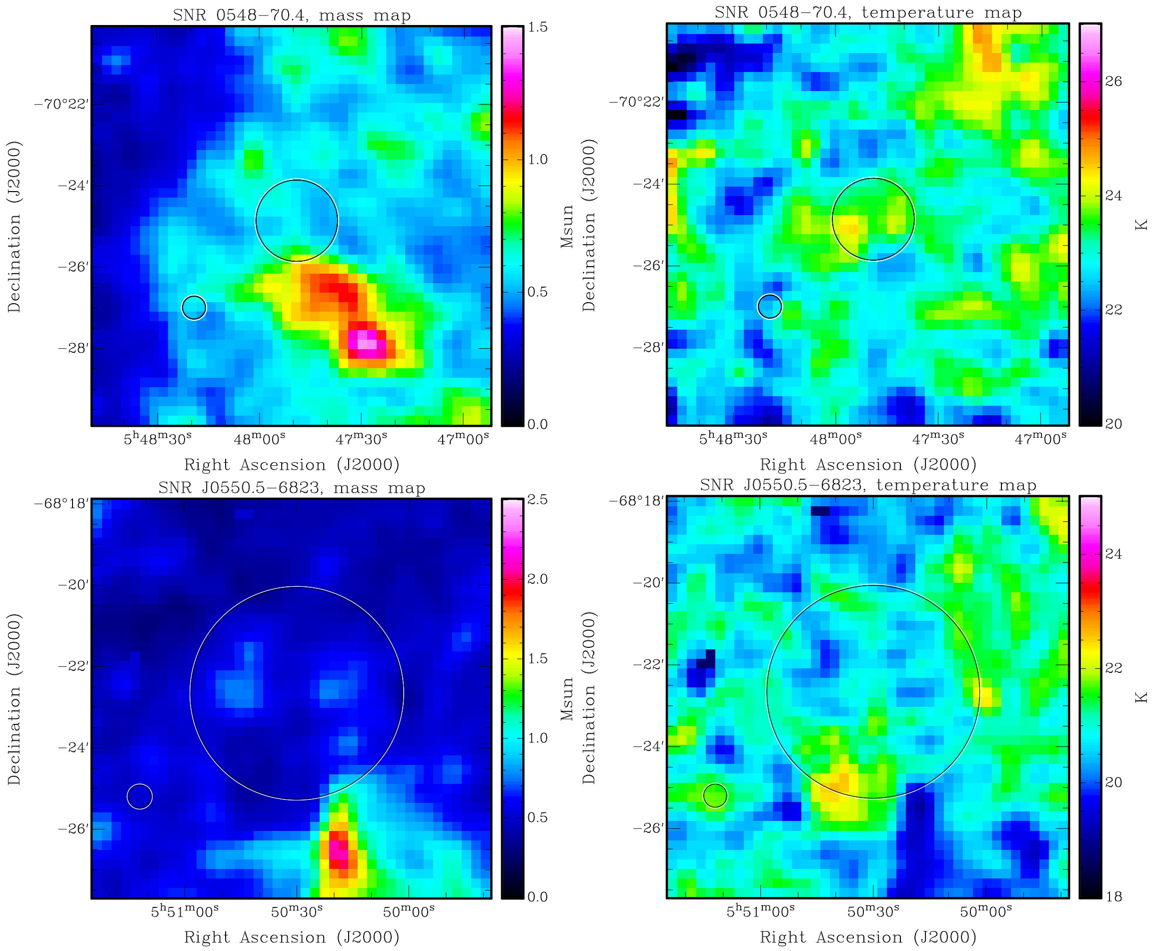


FIG. A.13.— 0548-70.4, and SNR J 0550.5−6823.
